# Supplementary material for: Enlarged Kuramoto Model: Secondary Instability and Transition to Collective Chaos
Source: arXiv:2112.00176 source file (2022-04-18)
Supplement: Supplementary file 1 [file sm5.pdf]

# Supplemental Material to “Enlarged Kuramoto Model: Secondary Instability and Transition to Collective Chaos”

Iván León and Diego Pazó  
*Instituto de Física de Cantabria (IFCA), Universidad de Cantabria-CSIC, 39005 Santander, Spain*

## CONTENTS

|      |                                        |   |
|------|----------------------------------------|---|
| I.   | Collective chaos in Eq. (1)            | 1 |
| II.  | Boundary of Incoherence for Eq. (1)    | 2 |
|      | Thermodynamic limit: Perturbed Density | 3 |
|      | Perturbation dynamics                  | 3 |
|      | Self-consistency condition             | 4 |
|      | Final result                           | 4 |
| III. | Derivation of Eq. (2)                  | 5 |
| IV.  | Boundary of Incoherence for Eq. (2)    | 6 |
|      | References                             | 6 |

## I. COLLECTIVE CHAOS IN EQ. (1)

The ensemble of heterogeneous Stuart-Landau oscillators (Eq. (1) in the main text) exhibits a wide variety of dynamical states. In this section we show the existence of collective chaos. Collective chaos is characterized by the existence of at least one positive Lyapunov exponent (LE) in the thermodynamic limit ( $N \rightarrow \infty$ ).

Verifying collective chaos in Eq. (1) is a hard task due to the unavoidable presence of microscopic (phase) chaos [1]. Microscopic chaos yields  $n_{mic} \gg 1$  positive LEs. Crucially, although  $n_{mic}$  is proportional to the system size  $N$ , the magnitude of the corresponding LEs decays to zero as  $N \rightarrow \infty$ . This means that for large enough  $N$ , the largest LE associated with collective chaos will prevail. Otherwise, if the largest LE decays to zero as  $N$  grows, then collective chaos can be ruled out.

In Fig. S1 we depict the largest LE  $\lambda$  versus the number of oscillators  $N$  for different parameter values. We choose  $c_2 = 3$ ,  $\sigma = 10^{-3}$ ,  $c_1 = -0.4$ , and  $\epsilon$  values as in Fig. 1 of the main text. Moreover, data for  $c_1 = -0.415$  and  $\epsilon = 0.14$  are also depicted. In the figure it can be observed that  $\lambda$  rapidly decays to zero for UIS (orange), PS (blue). This decaying is consistent with the  $1/N$  law reported in [1]. The exponent also decays to zero (although in a slower manner) for the parameters where the  $T^2$  is stable (gray). The LE computed for the largest  $\epsilon$  value in Fig. 1,  $\epsilon = 0.115$ , exhibits an even slower decay. This behavior does not confirm nor refute if (weak) collective chaos is already present. For a larger value of  $\epsilon = 0.14$  ( $c_1 = -0.415$ ), collective chaos is more evident, with  $\lambda \simeq 3.5 \times 10^{-4}$ . These values of  $\lambda$  are of the same order of magnitude than those found in the enlarged Kuramoto model with collective chaos, see Fig. 3(a).

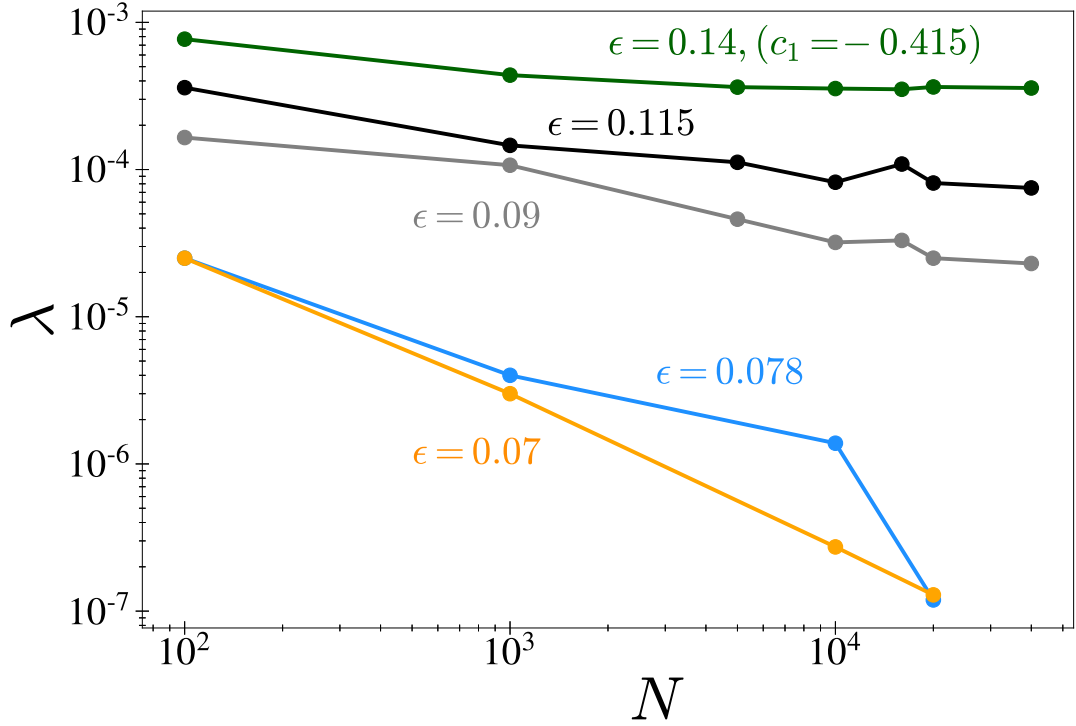

FIG. S1. Largest Lyapunov exponent for Eq. (1) in the main text as a function of the number of oscillators  $N$ . The parameter values are those used in Fig. 1 of the main text, namely  $c_1 = -0.4$ ,  $c_2 = 3$ ,  $\sigma = 10^{-3}$  and  $\epsilon = 0.07$  (orange),  $0.078$  (blue),  $0.09$  (gray), and  $0.115$  (black). Additionally, we selected  $\epsilon = 0.14$  and  $c_1 = -0.415$  (green) to show a state with clear-cut collective chaos.

## II. BOUNDARY OF INCOHERENCE FOR EQ. (1)

We derive the conditions satisfied at the marginal stability of incoherence for an infinite ensemble of Stuart-Landau oscillators, Eq. (1) in the main text. This derivation follows [2].

The outline of the derivation is as follows. First we consider an infinitesimal perturbation around the uniform incoherent state (UIS), written in terms of the density of oscillators. This perturbed density evolves according to the continuity equation, but in addition it should verify the self-consistent condition. That means, the distribution has to be consistent with the mean-field it produces. At the stability boundary of incoherence the perturbation neither decays nor grows.

For simplicity, it is convenient to transform the equation of the oscillators so that in the UIS the amplitude of the oscillations is 1. This can be achieved by a change of coordinates of the oscillators  $B_j = A_j \exp[i\epsilon c_1 t + i c_2(1 - \epsilon)t]/\sqrt{1 - \epsilon}$ , and rescaling time  $\tau = (1 - \epsilon)t$ , frequency  $\tilde{\omega} = \sigma\omega/(1 - \epsilon)$  and coupling

$$\kappa = \frac{\epsilon}{1 - \epsilon}. \quad (\text{S1})$$

In the new coordinates, Eq. (1) writes:

$$\frac{dB_j}{d\tau} = (1 + i\tilde{\omega}_j + i c_2)B_j - (1 + i c_2)|B_j|^2 B_j + \kappa(1 + i c_1)\bar{B}. \quad (\text{S2})$$

It is important to notice that now  $\tilde{\omega}$  are distributed following a Gaussian distribution  $g(\tilde{\omega})$  with standard deviation  $\tilde{\sigma} = \sigma/(1 - \epsilon) = \sigma(1 + \kappa)/(1 - \kappa)$ . This implies that the frequency distribution depends on  $\kappa$ . For convenience we write (S2) in polar coordinates:

$$\frac{dr_j}{d\tau} = \dot{r}_j = r_j - r_j^3 + \kappa|\bar{B}| [\cos(\Upsilon - \phi_j) - c_1 \sin(\Upsilon - \phi_j)], \quad (\text{S3})$$

$$\frac{d\phi_j}{d\tau} = \dot{\phi}_j = \tilde{\omega}_j + c_2(1 - r_j^2) + \frac{\kappa|\bar{B}|}{r_j} [\sin(\Upsilon - \phi_j) + c_1 \cos(\Upsilon - \phi_j)], \quad (\text{S4})$$

where the mean field is

$$\overline{B} \equiv |\overline{B}|e^{i\Upsilon}.$$

At UIS  $\overline{B} = 0$  and  $r_j = 1$ .

### Thermodynamic limit: Perturbed Density

As we are interested in the behavior in the thermodynamic limit  $N \rightarrow \infty$ , we can define the density distribution of oscillators  $\rho(r, \phi|\tilde{\omega}, \tau)$ , such that  $\rho(r, \phi|\tilde{\omega}, \tau)r d\phi dr$  is the fraction of oscillators between  $(r, r + dr)$  and  $(\phi, \phi + d\phi)$  with frequency  $\tilde{\omega}$  at time  $\tau$ . In the vicinity of the UIS the density is:

$$\rho(r, \phi|\tilde{\omega}, \tau) = \frac{1}{2\pi r} \delta[r - 1 - \varepsilon r_1(\phi|\tilde{\omega}, \tau)][1 + \varepsilon f_1(\phi|\tilde{\omega}, \tau)], \quad (\text{S5})$$

where the small constant  $\varepsilon$  explicits the smallness of the deviations from the unit circle and from the uniform angular density through  $r_1$  and  $f_1$ , respectively. Note that the normalization condition, requires the average of  $f_1$  over  $\phi$  to vanish.

$$1 = \int_0^\infty r dr \int_0^{2\pi} d\phi \rho = 1 + \frac{\varepsilon}{2\pi} \int_0^{2\pi} f_1(\phi|\tilde{\omega}, \tau) d\phi.$$

Close to the UIS, the amplitude of the mean field  $|\overline{B}|$  is a small quantity of order  $\varepsilon$ :

$$|\overline{B}| = \overline{B} e^{-i\Upsilon} = \int_{-\infty}^\infty d\tilde{\omega} g(\tilde{\omega}) \int_0^\infty r dr \int_0^{2\pi} d\phi \rho(r, \phi|\tilde{\omega}, \tau) r e^{i(\phi - \Upsilon)} = \frac{\varepsilon}{2\pi} \int_{-\infty}^\infty d\tilde{\omega} g(\tilde{\omega}) \int_0^{2\pi} d\phi [f_1(\phi|\tilde{\omega}, \tau) + r_1(\phi|\tilde{\omega}, \tau)] e^{i(\phi - \Upsilon)} + O(\varepsilon^2) \quad (\text{S6})$$

### Perturbation dynamics

The evolution of the radial perturbation  $r_1$  is obtained using the chain rule

$$\frac{dr}{d\tau} = \frac{\partial r}{\partial \phi} \frac{d\phi}{d\tau} + \frac{\partial r}{\partial \tau}. \quad (\text{S7})$$

Replacing (S3) and (S4) with  $r = 1 + \varepsilon r_1$ ,  $|\overline{B}| \equiv \varepsilon B_0$  and neglecting terms of order  $\varepsilon^2$ :

$$-2r_1 + \kappa B_0 [\cos(\Upsilon - \phi) - c_1 \sin(\Upsilon - \phi)] = \frac{\partial r_1}{\partial \phi} \tilde{\omega} + \frac{\partial r_1}{\partial \tau}. \quad (\text{S8})$$

We assume an exponential growth rate  $\lambda$  of the perturbation. In general,  $\lambda$  is a pure imaginary number at threshold, however, we assume  $\lambda$  is real provided the frequency distribution is shifted by a certain frequency shift  $\Omega_c$ , which is later obtained self-consistently. In this reference frame we can choose  $\Upsilon = 0$ , but we keep it for clarity. We replace  $\frac{\partial r_1}{\partial \tau}$  by  $= \lambda r_1$  in (S8). The solution has a trigonometric form:

$$r_1 = \kappa B_0 [\mathcal{A} \cos(\Upsilon - \phi) + \mathcal{B} \sin(\Upsilon - \phi)] \quad (\text{S9})$$

with

$$\mathcal{A} = \frac{2 + \lambda - c_1 \tilde{\omega}}{\tilde{\omega}^2 + (2 + \lambda)^2}, \quad \text{and} \quad \mathcal{B} = -\frac{(2 + \lambda)c_1 + \tilde{\omega}}{(2 + \lambda)^2 + \tilde{\omega}^2}.$$

Next, we calculate  $f_1$ . First of all notice that the density  $\rho$  satisfies the continuity equation:

$$\frac{\partial \rho}{\partial \tau} + \vec{\nabla} \cdot (\rho \vec{v}) = 0, \quad (\text{S10})$$

where  $\vec{v}$  is the velocity vector. The divergence in polar coordinates is  $\vec{\nabla} \cdot \vec{F} = \frac{1}{r} \frac{\partial}{\partial r} (r F_r) + \frac{1}{r} \frac{\partial F_\phi}{\partial \phi}$  with  $\vec{F} = F_r \vec{u}_r + F_\phi \vec{u}_\phi$ . In our case  $F_r = \rho \dot{r}$  and  $F_\phi = \rho r \dot{\phi}$ . We integrate Eq. (S10) over  $r$ :

$$\varepsilon \frac{\partial f_1}{\partial \tau} + \int_0^\infty dr \left\{ (1 + \varepsilon f_1) \partial_r [\dot{r} \delta(r - 1 - \varepsilon r_1)] + \delta(r - 1 - \varepsilon r_1) \partial_\phi [\dot{\phi} (1 + \varepsilon f_1)] \right\} = 0. \quad (\text{S11})$$

Now, we replace  $\frac{\partial f_1}{\partial \tau}$  by  $\lambda f_1$  and keep only the order  $\varepsilon$  terms:

$$\lambda f_1 + \tilde{\omega} \frac{\partial f_1}{\partial \phi} - 2c_2 \frac{\partial r_1}{\partial \phi} + \kappa B_0 \frac{\partial}{\partial \phi} [c_1 \cos(\Upsilon - \phi) + \sin(\Upsilon - \phi)] = 0 \quad (\text{S12})$$

and using  $r_1$  from Eq. (S9):

$$\tilde{\omega} \partial_\phi f_1 = -\lambda f_1 + \kappa B_0 [(1 - 2c_2 B) \cos(\Upsilon - \phi) + (2c_2 A - c_1) \sin(\Upsilon - \phi)].$$

If  $f_1(\phi|\tilde{\omega}) = \kappa B_0 [\mathcal{C} \cos(\Upsilon - \phi) + \mathcal{D} \sin(\Upsilon - \phi)]$ :

$$\tilde{\omega} \mathcal{C} + \lambda \mathcal{D} = 2c_2 \mathcal{A} - c_1, \quad (\text{S13})$$

$$\lambda \mathcal{C} - \tilde{\omega} \mathcal{D} = 1 - 2c_2 \mathcal{B}. \quad (\text{S14})$$

The solutions are:

$$\mathcal{C} = \frac{(1 + c_1 c_2) \lambda + \tilde{\omega} (c_2 - c_1)}{\lambda^2 + \tilde{\omega}^2} - \frac{c_2 [c_1 (\lambda + 2) + \tilde{\omega}]}{(\lambda + 2)^2 + \tilde{\omega}^2} \quad ; \quad \mathcal{D} = -\frac{(1 + c_1 c_2) \tilde{\omega} + (c_1 - c_2) \lambda}{\lambda^2 + \tilde{\omega}^2} - \frac{c_2 (\lambda + 2 - c_1 \tilde{\omega})}{[\lambda + 2(1 - \epsilon)]^2 + \tilde{\omega}^2}.$$

### Self-consistency condition

Our solutions for  $f_1$  and  $r_1$  must be consistent with Eq. (S6) (self-consistency condition). This implies:

$$2\pi = \int_{-\infty}^{\infty} d\tilde{\omega} g(\tilde{\omega}) \int_0^{2\pi} d\phi e^{i(\phi - \Upsilon)} (r_1 + f_1) / B_0 = \kappa \int_{-\infty}^{\infty} d\tilde{\omega} g(\tilde{\omega}) \int_0^{2\pi} d\phi e^{i(\phi - \Upsilon)} [(\mathcal{A} + \mathcal{C}) \cos(\Upsilon - \phi) + (\mathcal{B} + \mathcal{D}) \sin(\Upsilon - \phi)].$$

This yields two equations for the imaginary and real parts, respectively:

$$\int_{-\infty}^{\infty} d\tilde{\omega} g(\tilde{\omega}) (\mathcal{B} + \mathcal{D}) = 0, \quad (\text{S15})$$

$$\kappa \int_{-\infty}^{\infty} d\tilde{\omega} g(\tilde{\omega}) (\mathcal{A} + \mathcal{C}) = 2. \quad (\text{S16})$$

### Final result

For the stability threshold, we make  $\lambda \rightarrow 0$ :

$$\mathcal{A}(\lambda \rightarrow 0) = \frac{2 - c_1 \tilde{\omega}}{\tilde{\omega}^2 + 4}, \quad (\text{S17})$$

$$\mathcal{B}(\lambda \rightarrow 0) = -\frac{2c_1 + \tilde{\omega}}{\tilde{\omega}^2 + 4}, \quad (\text{S18})$$

$$\mathcal{C}(\lambda \rightarrow 0) = \pi(1 + c_1 c_2) \delta(\tilde{\omega}) + \frac{(c_2 - c_1) \tilde{\omega}}{\tilde{\omega}^2 + \lambda^2} - \frac{c_2 (2c_1 + \tilde{\omega})}{\tilde{\omega}^2 + 4}, \quad (\text{S19})$$

$$\mathcal{D}(\lambda \rightarrow 0) = \pi(c_2 - c_1) \delta(\tilde{\omega}) - \frac{(1 + c_1 c_2) \tilde{\omega}}{\tilde{\omega}^2 + \lambda^2} + \frac{c_1 c_2 \tilde{\omega} - 2c_2}{\tilde{\omega}^2 + 4}. \quad (\text{S20})$$

To obtain the boundary of incoherence we need the  $\kappa_c$ - and  $\Omega_c$ -dependent integrals:

$$I_1 = \int d\tilde{\omega} \frac{g(\tilde{\omega})}{\tilde{\omega}^2 + 4}; \quad I_2 = \lim_{\lambda \rightarrow 0} \int d\tilde{\omega} \frac{g(\tilde{\omega}) \tilde{\omega}}{\tilde{\omega}^2 + \lambda^2} = p.v. \int g(\tilde{\omega}) \frac{d\tilde{\omega}}{\tilde{\omega}} d\tilde{\omega}; \quad I_3 = \int d\tilde{\omega} \frac{g(\tilde{\omega}) \tilde{\omega}}{\tilde{\omega}^2 + 4}; \quad I_4 = \int d\tilde{\omega} g(\tilde{\omega}) \delta(\tilde{\omega}) = g(0) \quad (\text{S21})$$

We have then:

$$-2(c_1 + c_2) I_1 - (1 + c_1 c_2) I_2 - (1 - c_1 c_2) I_3 + \pi(c_2 - c_1) I_4 = 0 \quad (\text{S22})$$

$$2(1 - c_1 c_2) I_1 + (c_2 - c_1) I_2 - (c_1 + c_2) I_3 + \pi(1 + c_1 c_2) I_4 = 2/\kappa_c \quad (\text{S23})$$

This equation determine the boundary of the UIS and the frequency of the instability  $\Omega_c$ . The most efficient way to compute the stability boundary is to fix  $\kappa_c$  and  $\Omega_c$ , compute  $I_i$  and use (S22) and (S23) to obtain  $c_1$  and  $c_2$ . Finally, one refers to Eq. (S1) to obtain  $\epsilon_c$ .

### III. DERIVATION OF EQ. (2)

In this section we apply second order phase reduction to the ensemble of globally coupled Stuart-Landau oscillators, Eq. (1). Neglecting terms of order  $O(\epsilon^3)$  and  $O(\epsilon^2\sigma)$  we obtain Eq. (2) in the main text.

The first step in phase reduction is performing a change of variable in Eq. (1) to phase and amplitude,  $A_j = r_j e^{i(\theta_j + c_2 \ln r_j)}$ . Additionally, we go to a rotating reference frame such that the frequency of the oscillator is  $\sigma\omega_j$ :

$$\dot{r}_j = r_j(1 - \epsilon - r_j^2) + \frac{\epsilon\Gamma}{N} \sum_{k=1}^N r_k \left\{ \sin [\theta_k - \theta_j + \gamma + c_2(\ln r_k - \ln r_j)] \right\} \quad (\text{S24a})$$

$$\dot{\theta}_j = \sigma\omega_j + \frac{\epsilon\eta}{Nr_j} \sum_{k=1}^N r_k \left\{ \sin [\theta_k - \theta_j + \alpha + c_2(\ln r_k - \ln r_j)] \right\}, \quad (\text{S24b})$$

where, for simplicity, we have defined  $\Gamma = \sqrt{1 + c_1^2}$ ,  $\tan \gamma = -1/c_1$ , and  $\eta$  and  $\alpha$  as in the main text.

Assuming the smallness of the coupling parameter  $\epsilon$  we can expand the radial variable in this parameter  $r_j = 1 + \epsilon r_j^{(1)} + \epsilon^2 r_j^{(2)} + \dots$  where the zeroth order is 1 since the limit cycle has  $r = 1$ . To obtain the second-order phase reduction we expand the equation (S24b) up to order  $\epsilon^2$ :

$$\dot{\theta}_j = \sigma\omega_j + \frac{\epsilon\eta}{N} \sum_{k=1}^N \sin(\theta_k - \theta_j + \alpha) + \epsilon^2 \eta \sqrt{(1 + c_2^2)} \left[ \frac{1}{N} \sum_{k=1}^N r_k^{(1)} \sin(\theta_k - \theta_j + \alpha + \delta) - \frac{1}{N} r_j^{(1)} \sum_{k=1}^N \sin(\theta_k - \theta_j + \alpha + \delta) \right] + O(\epsilon^3) \quad (\text{S25})$$

or

$$\dot{\theta}_j = \sigma\omega_j + \epsilon\eta R \sin(\Psi - \theta_j + \alpha) + \epsilon^2 \eta \sqrt{(1 + c_2^2)} \left[ \frac{1}{N} \sum_{k=1}^N r_k^{(1)} \sin(\theta_k - \theta_j + \alpha + \delta) - r_j^{(1)} R \sin(\Psi - \theta_j + \alpha + \delta) \right] + O(\epsilon^3) \quad (\text{S26})$$

where  $\tan \delta = c_2$ . Now, to close this equation we only need the radial correction up the order  $\epsilon$ , i.e.  $r_j^{(1)}$ .

In order to obtain  $r_j^{(1)}$  we assume the radii depend on the phases,  $r_j = r_j(\theta)$ , and apply the chain rule to (S24a),  $\dot{r}_j = \sum_k \dot{\theta}_k \partial_{\theta_k} r_j$ . Expanding  $r_j$  in powers of  $\epsilon$ , we obtain the equation for  $r_j^{(1)}$ :

$$\sum_{k=1}^N \sigma\omega_k \partial_{\theta_k} r_j^{(1)} = -2r_j^{(1)} + \frac{\Gamma}{N} \sum_{k=1}^N \sin(\theta_k - \theta_j + \gamma), \quad (\text{S27})$$

whose solution is

$$r_j^{(1)} = \frac{\Gamma}{N} \sum_{k=1}^N \frac{1}{2 + \sigma^2 \frac{(\omega_k - \omega_j)^2}{2}} \sin(\theta_k - \theta_j + \gamma) - \sigma \frac{\omega_k - \omega_j}{4 + \sigma^2 (\omega_k - \omega_j)^2} \cos(\theta_k - \theta_j + \gamma). \quad (\text{S28})$$

Neglecting terms of order  $\sigma$ :

$$r_j^{(1)} \simeq \frac{\Gamma}{2} R \sin(\Psi - \theta_j + \gamma) \quad (\text{S29})$$

Replacing (S29) into the (S26) and using the relations  $\alpha + \delta + \gamma = \beta - \pi/2$  and  $-\alpha - \delta + \gamma = -\pi/2$  we obtain Eq. (2) in the main text. Notice that preserving the  $O(\sigma)$  term of (S28) translates into an  $O(\epsilon^2\sigma)$  term in Eq. (S26). This term is safely neglected provided that  $\sigma \ll 1$ . The relative importance of terms  $O(\epsilon^2\sigma)$  and  $O(\epsilon^3)$  depends on the ratio  $\epsilon/\sigma$ . In conclusion, Eq. (2) in the main text is the phase reduction of Eq. (1) after neglecting terms  $O(\epsilon^3)$  and  $O(\epsilon^2\sigma)$ .

#### IV. BOUNDARY OF INCOHERENCE FOR EQ. (2)

This section is devoted to deriving the boundary of the uniform incoherent state (UIS) in the enlarged Kuramoto model, Eq. (2) in the main text. In order to compute this boundary we first note that in the neighborhood of UIS ( $R = Q = 0$ ) nonlinear terms in  $R$  and  $Q$  are negligible. Removing these nonlinear terms in the enlarged Kuramoto model, Eq. (2) in the main text, we get the classical Kuramoto-Sakaguchi model:

$$\dot{\theta}_j = \epsilon \eta R \sin(\psi - \theta_j + \alpha) + \frac{\epsilon^2 \eta^2}{4} R \sin(\psi - \theta_j + \beta) = \epsilon \hat{\eta} R \sin(\psi - \theta_j - \hat{\alpha}), \quad (\text{S30})$$

where

$$\hat{\eta} = \eta \sqrt{1 + \frac{\epsilon}{2}(1 - c_1 c_2) + \frac{\epsilon^2}{4} \eta^2}, \quad (\text{S31})$$

$$\hat{\alpha} = \arg \left\{ 1 + c_1 c_2 + \frac{\epsilon}{4}(1 + c_2^2)(1 - c_1^2) + i \left[ c_1 - c_2 + \frac{\epsilon c_1}{2}(1 + c_2^2) \right] \right\}. \quad (\text{S32})$$

The transition point between UIS and partial synchrony, for a symmetric frequency distribution, satisfies [3]:

$$\epsilon_c \hat{\eta} = \frac{2 \cos \hat{\alpha}}{\pi g(\Omega_c)}, \quad (\text{S33a})$$

$$PV(\Omega_c) = \frac{\pi g(\Omega_c) \tan \hat{\alpha}}{2}, \quad (\text{S33b})$$

where  $\Omega_c$  is the critical frequency at the onset of partial synchronization, which remains to be determined. The function  $PV(\Omega)$  in (S33b) is defined as

$$PV(\Omega) = \lim_{a \rightarrow 0} \left( \int_{-\infty}^{-\Omega-a} + \int_{-\Omega+a}^{\infty} \right) \frac{g(\omega)}{2(\omega - \Omega)} d\omega = p.v. \int_{-\infty}^{\infty} \left[ \frac{g(\omega)}{2(\omega - \Omega)} \right] d\omega. \quad (\text{S34})$$

We can now express (S33) in terms of  $c_1$ ,  $c_2$  and  $\epsilon_c$

$$\frac{\pi g(\Omega_c)}{2} = \frac{1 + c_1 c_2 + \frac{\epsilon_c}{4}(1 + c_2^2)(1 - c_1^2)}{\epsilon_c \{ (1 + c_1^2)(1 + c_2^2) [1 + \frac{\epsilon_c}{2}(1 - c_1 c_2) + \frac{\epsilon_c^2}{4} \eta^2] \}}, \quad (\text{S35a})$$

$$\frac{2PV(\Omega_c)}{\pi g(\Omega_c)} = \frac{c_1 - c_2 + \frac{\epsilon_c c_1}{2}(1 + c_2^2)}{1 + c_1 c_2 + \frac{\epsilon_c}{4}(1 + c_2^2)(1 - c_1^2)}. \quad (\text{S35b})$$

From these equations, we numerically compute the UIS boundary in Fig. 2(c).

- 
- [1] O. V. Popovych, Y. L. Maistrenko, and P. A. Tass, “Phase chaos in coupled oscillators,” *Phys. Rev. E* **71**, 065201(R) (2005).  
 [2] M. C. Cross, J. L. Rogers, R. Lifshitz, and A. Zumdieck, “Synchronization by reactive coupling and nonlinear frequency pulling,” *Phys. Rev. E* **73**, 036205 (2006).  
 [3] H. Sakaguchi and Y. Kuramoto, “A soluble active rotator model showing phase transitions via mutual entrainment,” *Prog. Theor. Phys.* **76**, 576–581 (1986).
